# Supplementary material for: Interplay between growth conditions and formation of localized light emitters in epitaxial AlN thin films
Source: arXiv:2609.12772 source file (2026-09-11)
Supplement: Supplementary file 1 [file SuppMat.tex]

\documentclass[%
 reprint,
 onecolumn,
superscriptaddress,
%groupedaddress,
%unsortedaddress,
%runinaddress,
%frontmatterverbose, 
%preprint,
%preprintnumbers,
%nofootinbib,
%nobibnotes,
%bibnotes,
 amsmath,amssymb,
 aps,
prapplied,
%prb,
%rmp,
%prstab,
%prstper,
%floatfix,
]{revtex4-2}

%%%%%%%%%%%%%%%%%%%%%%%%%%%%%%%%%%%%%%
%Include packages
\usepackage{graphicx}% Include figure files
%\usepackage{dcolumn}% Align table columns on decimal point
%\usepackage{bm}% bold math
%\usepackage{float}  % Add this line
\usepackage{xcolor}
\usepackage[colorlinks=true, allcolors=blue]{hyperref}

%%%%%%%%%%%%%%%%%%%%%%%%%%%%%%%%%%%%%%
%Renew figure and equation labels
\renewcommand{\thefigure}{S\arabic{figure}}
\renewcommand{\theequation}{S\arabic{equation}}
\renewcommand{\thesection}{S\arabic{section}}


%%%%%%%%%%%%%%%%%%%%%%%%%%%%%%%%%%%%%%
%New commands and definitions
\newcommand{\wnmbr}[0]{\mathrm{cm}^{-1}}
\newcommand{\um}[0]{\mu\mathrm{m}}

%%%%%%%%%%%%%%%%%%%%%%%%%%%%%%%%%%%%%%
%Text color commands
\newcommand{\red}[1]{{\color{red}#1}}
\newcommand{\blue}[1]{{\color{blue}#1}}


\begin{document}

%\preprint{}

\title{Interplay between growth conditions and formation of localized light emitters in epitaxial AlN thin films} 

\author{Meysam Saeedi}
\affiliation{Paul-Drude-Institut für Festkörperelektronik, Leibniz-Institut im Forschungsverbund Berlin e.V., Hausvogteiplatz 5-7, 10117 Berlin, Germany}

\author{Duc V. Dinh}
\affiliation{Paul-Drude-Institut für Festkörperelektronik, Leibniz-Institut im Forschungsverbund Berlin e.V., Hausvogteiplatz 5-7, 10117 Berlin, Germany}

\author{Andrey N. Anisimov}
\affiliation{Helmholtz-Zentrum Dresden-Rossendorf, Institute of Ion Beam Physics and Materials Research, Bautzner Landstrasse 400, 01328 Dresden, Germany}

\author{Mingyun Yuan}
\affiliation{Paul-Drude-Institut für Festkörperelektronik, Leibniz-Institut im Forschungsverbund Berlin e.V., Hausvogteiplatz 5-7, 10117 Berlin, Germany}

\author{Georgy V. Astakhov}
\affiliation{Helmholtz-Zentrum Dresden-Rossendorf, Institute of Ion Beam Physics and Materials Research, Bautzner Landstrasse 400, 01328 Dresden, Germany}

\author{Alberto Hernández-Mínguez}
\email{hernandez-minguez@pdi-berlin.de}
\affiliation{Paul-Drude-Institut für Festkörperelektronik, Leibniz-Institut im Forschungsverbund Berlin e.V., Hausvogteiplatz 5-7, 10117 Berlin, Germany}

\date{\today}% It is always \today, today,
             %  but any date may be explicitly specified

\begin{abstract}
This Supplemental Material contains information about:
\begin{itemize}
\item X-ray diffraction measurements of as-grown AlN thin films.
\item Proton irradiation calculations.
\item Effect of post-growth treatment on broadband PL emission.
\end{itemize}
\end{abstract}

\maketitle

\newpage

%%%%%%%%%%%%%%%%%%%%%%%%%%%%%%%%%%%%%%%%%%%%%%%%%%%%%%%%%%%%%%%%%%%%%%%%%%%%%%%%%%%%%%%%%%
\section{X-ray diffraction measurements of as-grown AlN thin films}

To determine the crystalline quality of the as-grown AlN thin films, we performed X-ray diffraction (XRD) measurements. Figure~\ref{fig:XRD}(a) displays the symmetric $2\theta-\omega$ XRD scans of the samples grown under N-rich and Al-rich conditions (dark green and violet curves, respectively). In addition to the peaks related to the 4H-SiC substrate, both XRD scans show two additional diffraction peaks corresponding to the 0002 and 0004 reflections of wurtzite AlN. Figure~\ref{fig:XRD}(b) compares the $\omega$ scans of the AlN 0002 peak in both samples. The AlN thin film grown under Al-rich conditions exhibits better crystallinity -- evidenced by the higher intensity and smaller line width -- compared to the AlN thin film grown under N-rich conditions.

\begin{figure}[h]
    \includegraphics[width=0.4\textwidth]{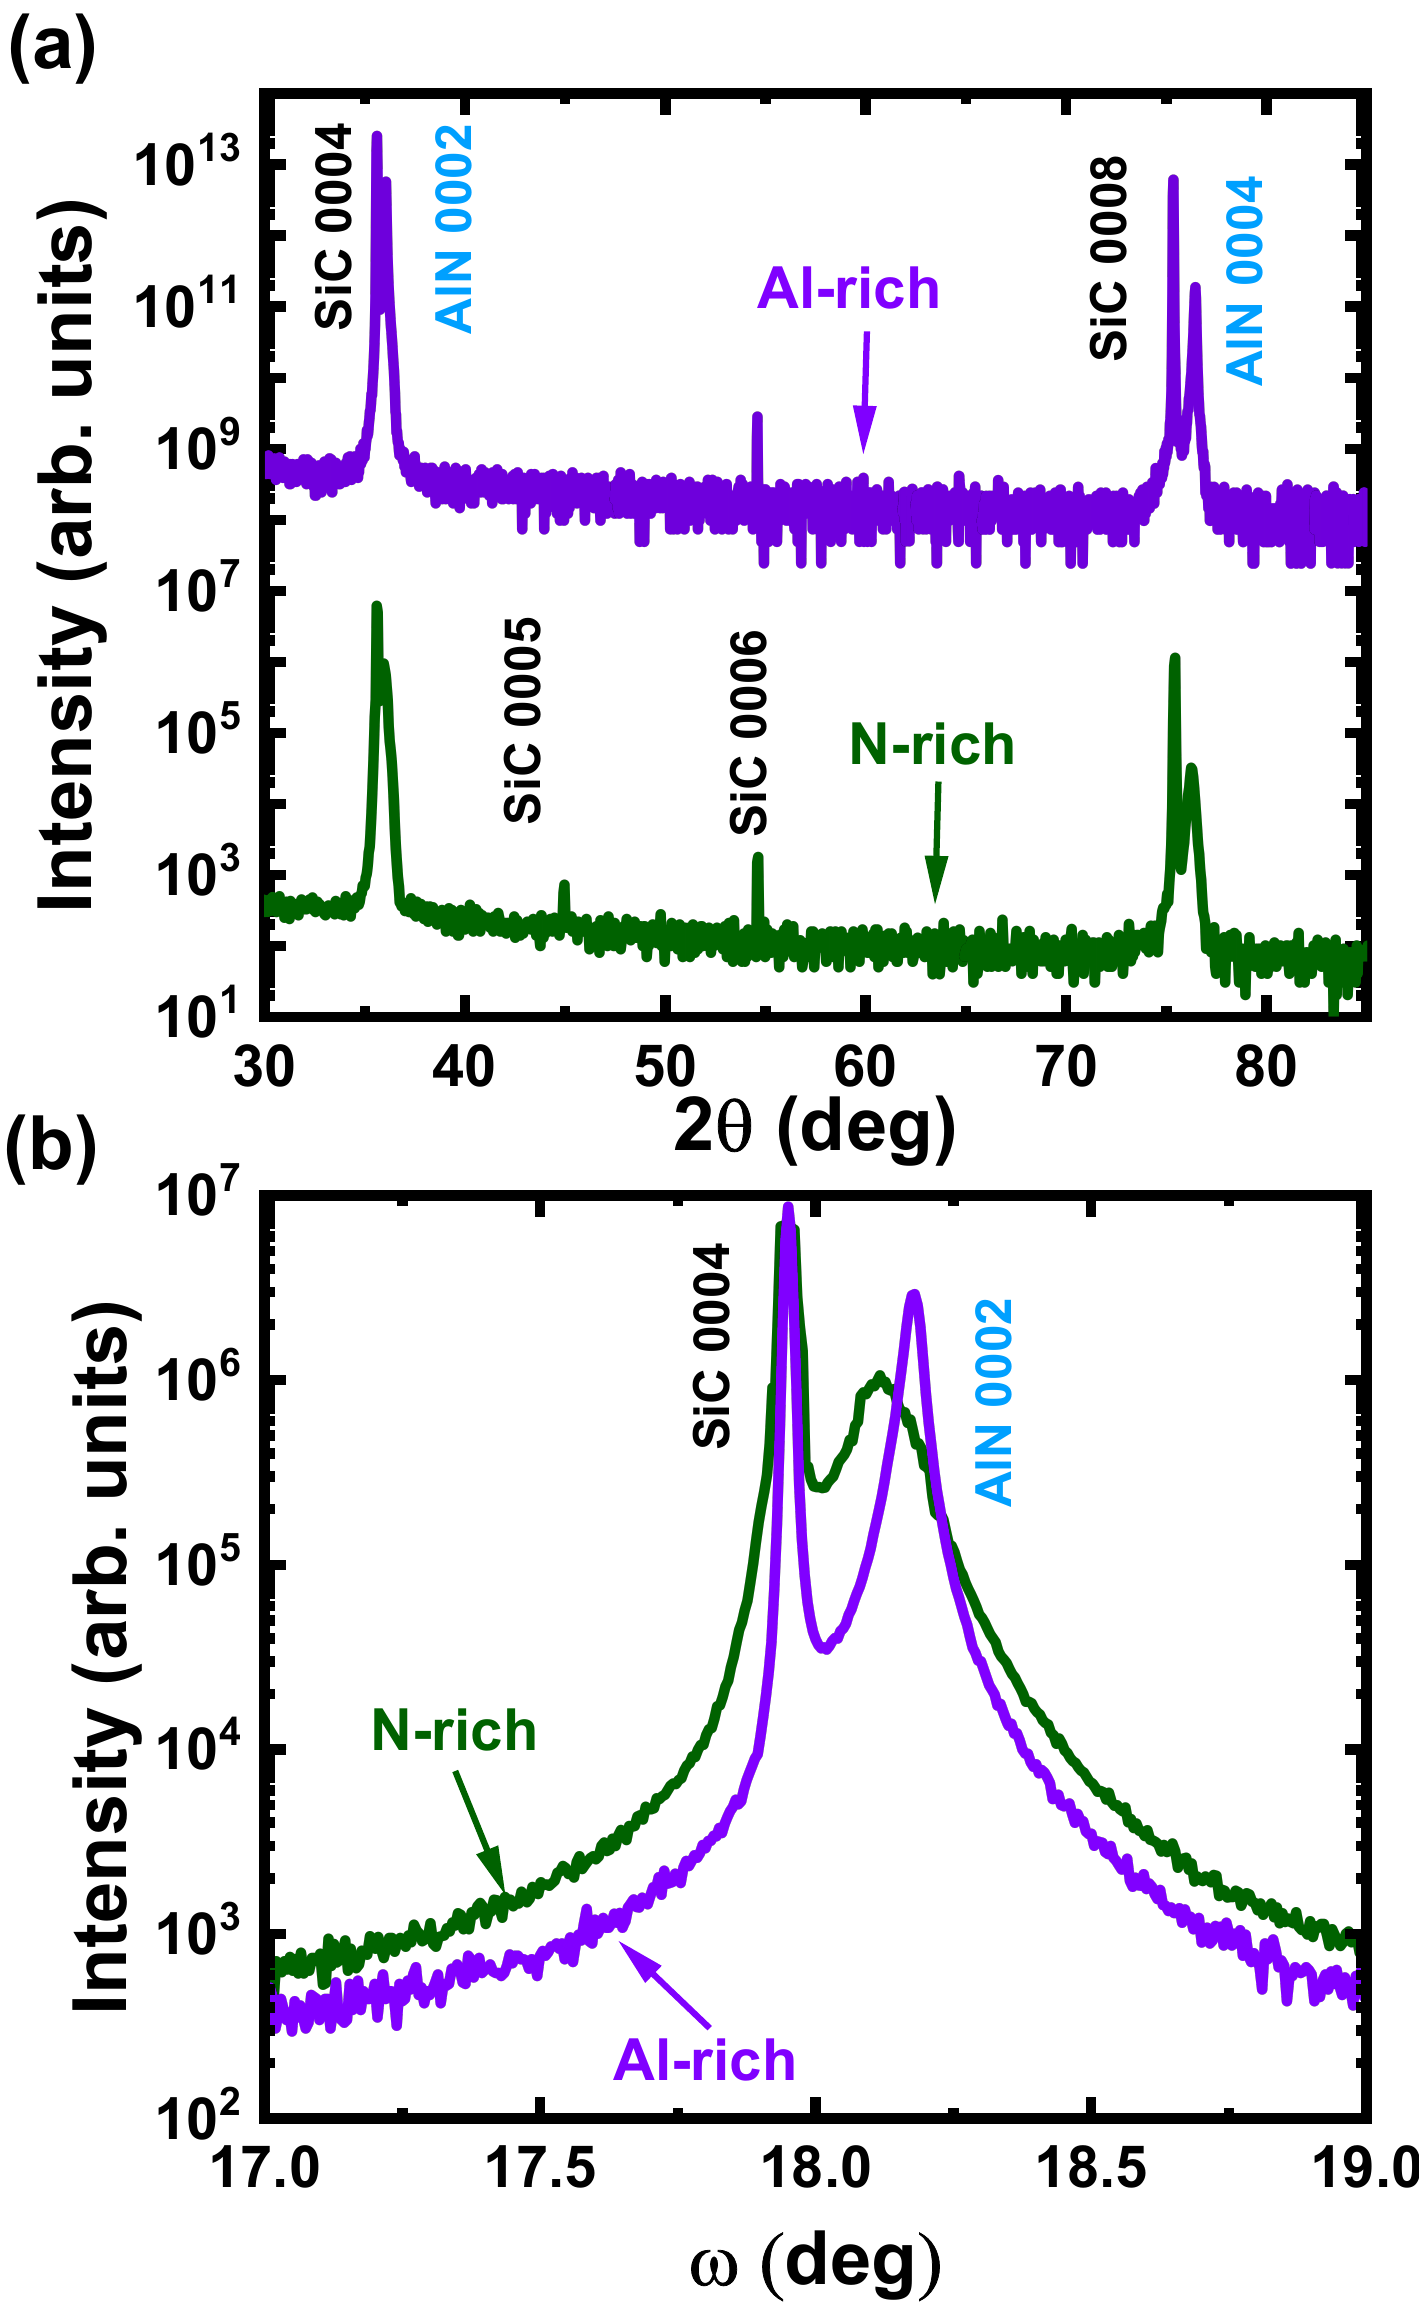}
    \caption{\label{fig:XRD}
    (a) Symmetric $2\theta-\omega$ X-ray diffraction scans of the as-grown AlN thin films. The dark green and violet curves correspond to the samples grown under N-rich and Al-rich conditions, respectively. The curves are vertically shifted for clarity.
    (b) Comparison of the $\omega$ scan for the AlN 0002 peak in both samples.
    }
\end{figure}

\newpage

%%%%%%%%%%%%%%%%%%%%%%%%%%%%%%%%%%%%%%%%%%%%%%%%%%%%%%%%%%%%%%%%%%%%%%%%%%%%%%%%%%%%%%%%%%
\section{Proton irradiation calculations}

Figure~\ref{fig:IrrSim}(a) shows the simulated depth profile of the density of protons scattered by the crystal lattice of AlN, calculated for a proton fluence and energy of $10^{15}$~cm$^{-2}$ and 60~keV, respectively. Figure~\ref{fig:IrrSim}(b) shows the estimated depth profiles of Al and N vacancies ($\mathrm{V_{Al}}$ and $\mathrm{V_N}$, respectively) formed in the proton irradiation process. The irradiation parameters were selected to form the maximum density of vacancies around the middle thickness of the AlN thin film.

\begin{figure}[h]
    \includegraphics[width=0.4\textwidth]{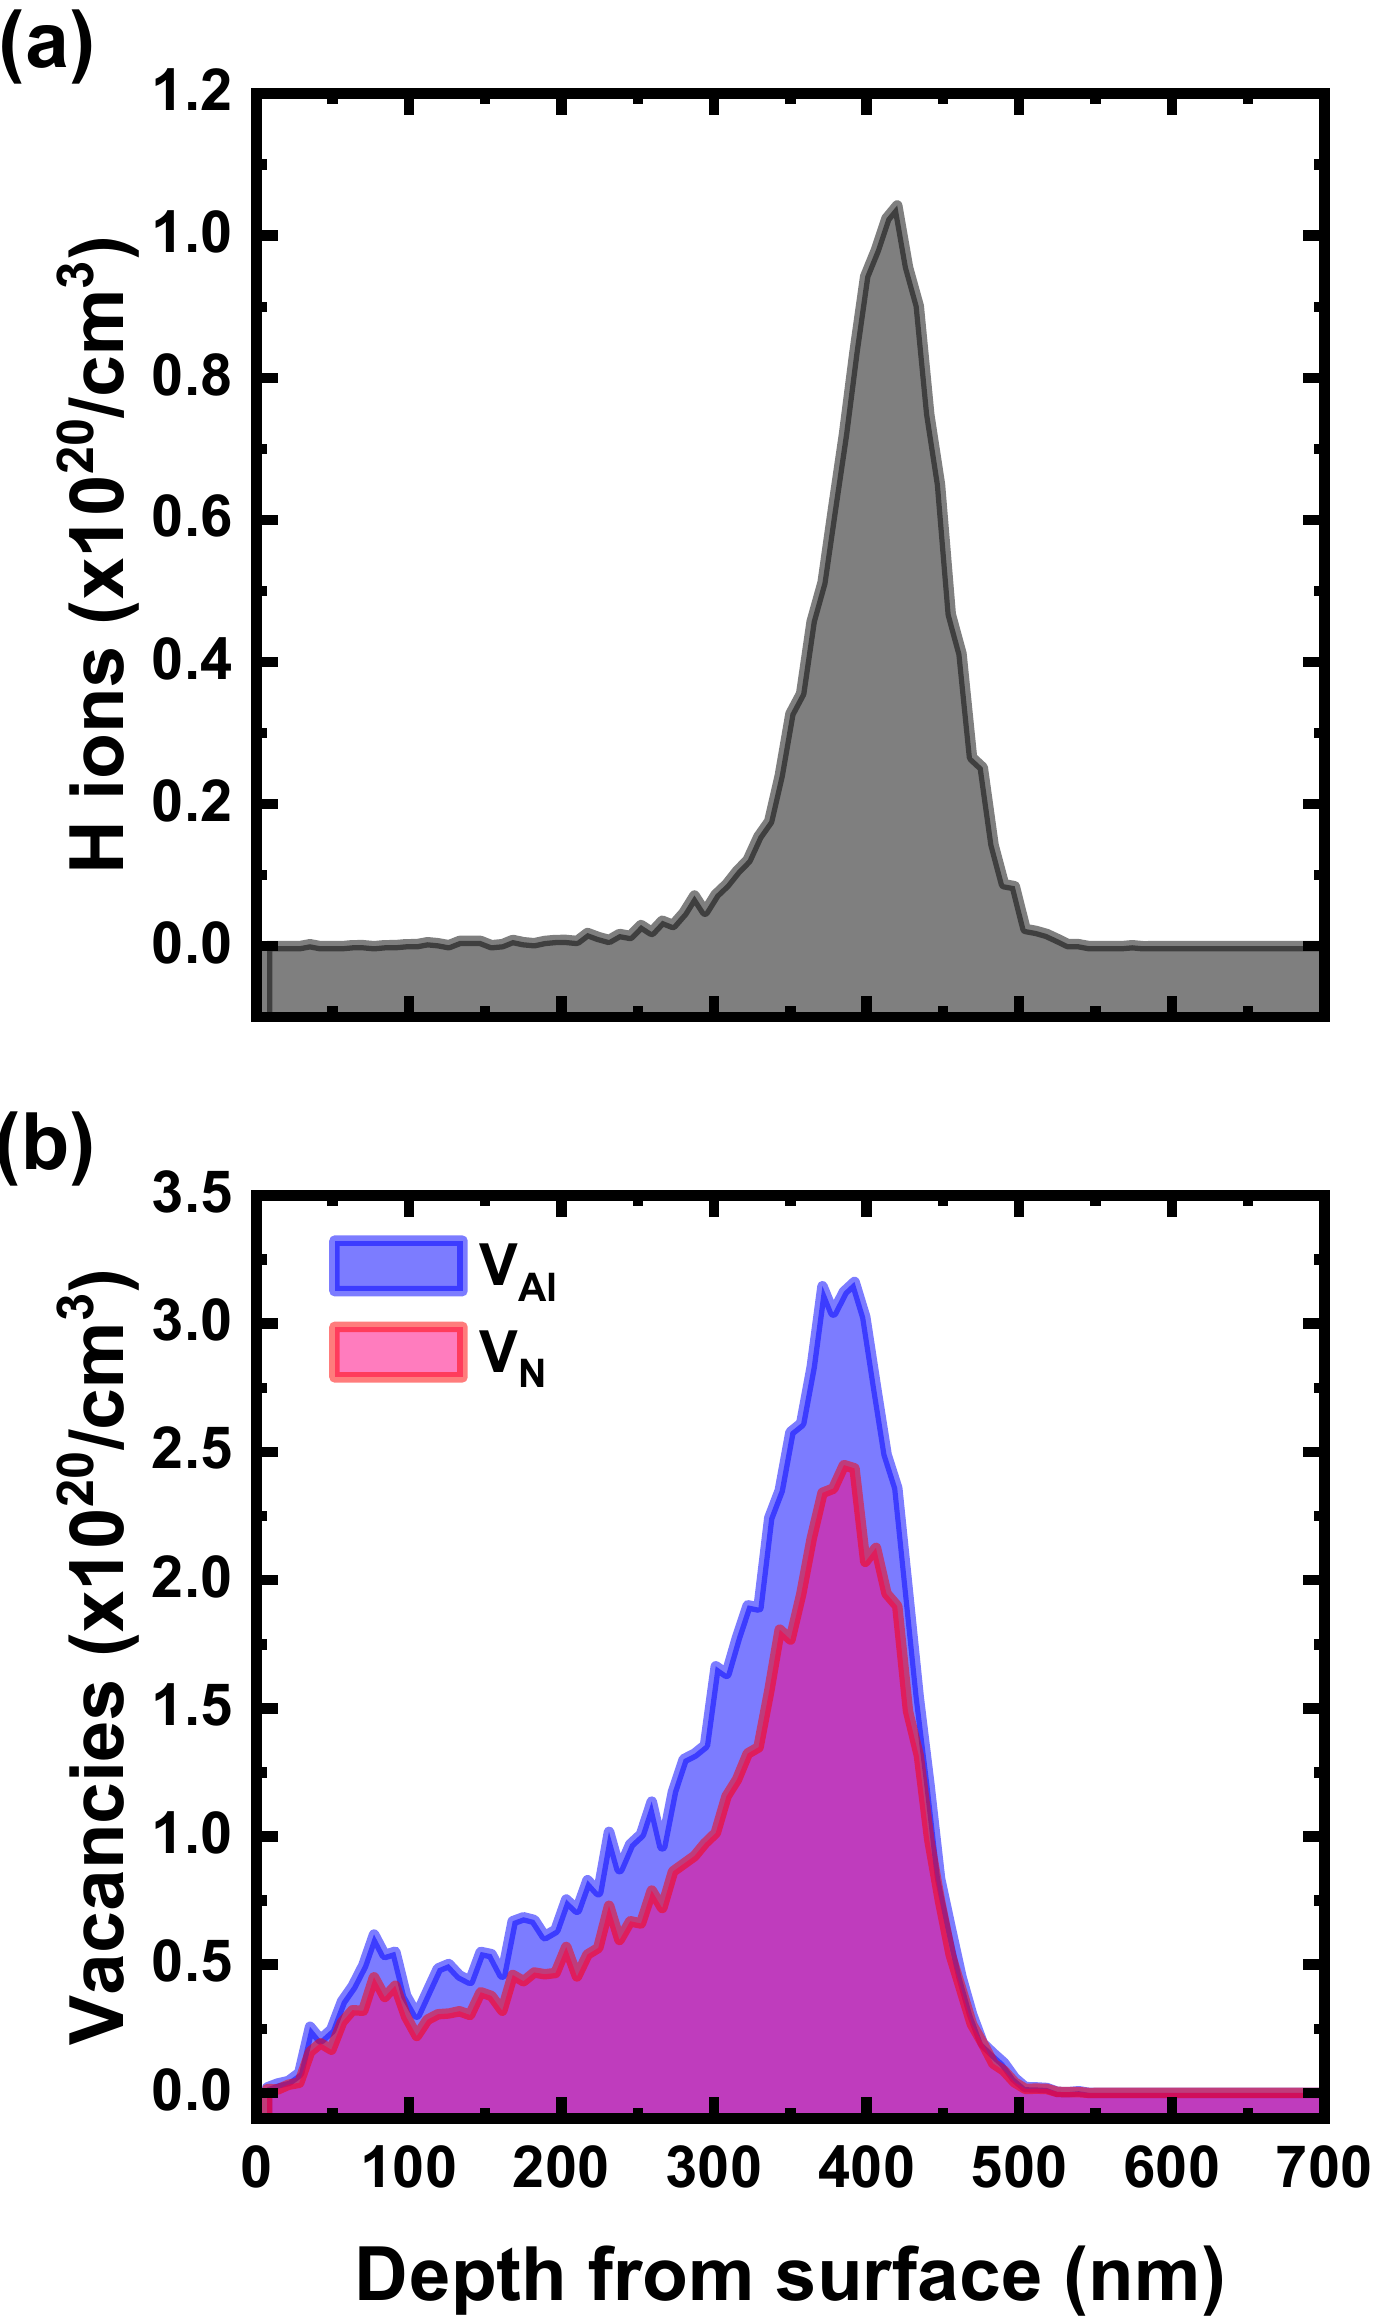}
    \caption{\label{fig:IrrSim}
    (a) Calculated depth dependence of the density of protons scattered by the AlN crystal atoms. 
    (b) Estimated depth profiles of the densities of $\mathrm{V_{Al}}$ and $\mathrm{V_N}$ formed by the proton irradiation.
    }
\end{figure}

\newpage

%%%%%%%%%%%%%%%%%%%%%%%%%%%%%%%%%%%%%%%%%%%%%%%%%%%%%%%%%%%%%%%%%%%%%%%%%%%%%%%%%%%%%%%%%%
\section{Effect of post-growth treatment on broadband PL emission}

Figure~\ref{fig:PL_Broad} compares the broad PL emission of the AlN thin films before and after proton irradiation and annealing. The broad PL of the film grown under N-rich conditions is about ten times brighter than the broad PL of the film grown under Al-rich conditions, cf. dark green and dark purple curves in Figs.~\ref{fig:PL_Broad}(a) and \ref{fig:PL_Broad}(b), respectively. After proton irradiation and annealing, the intensity of the broad PL reduces in both samples, cf. dark and bright curves in both panels.

\begin{figure}[h]
    \includegraphics[width=0.5\textwidth]{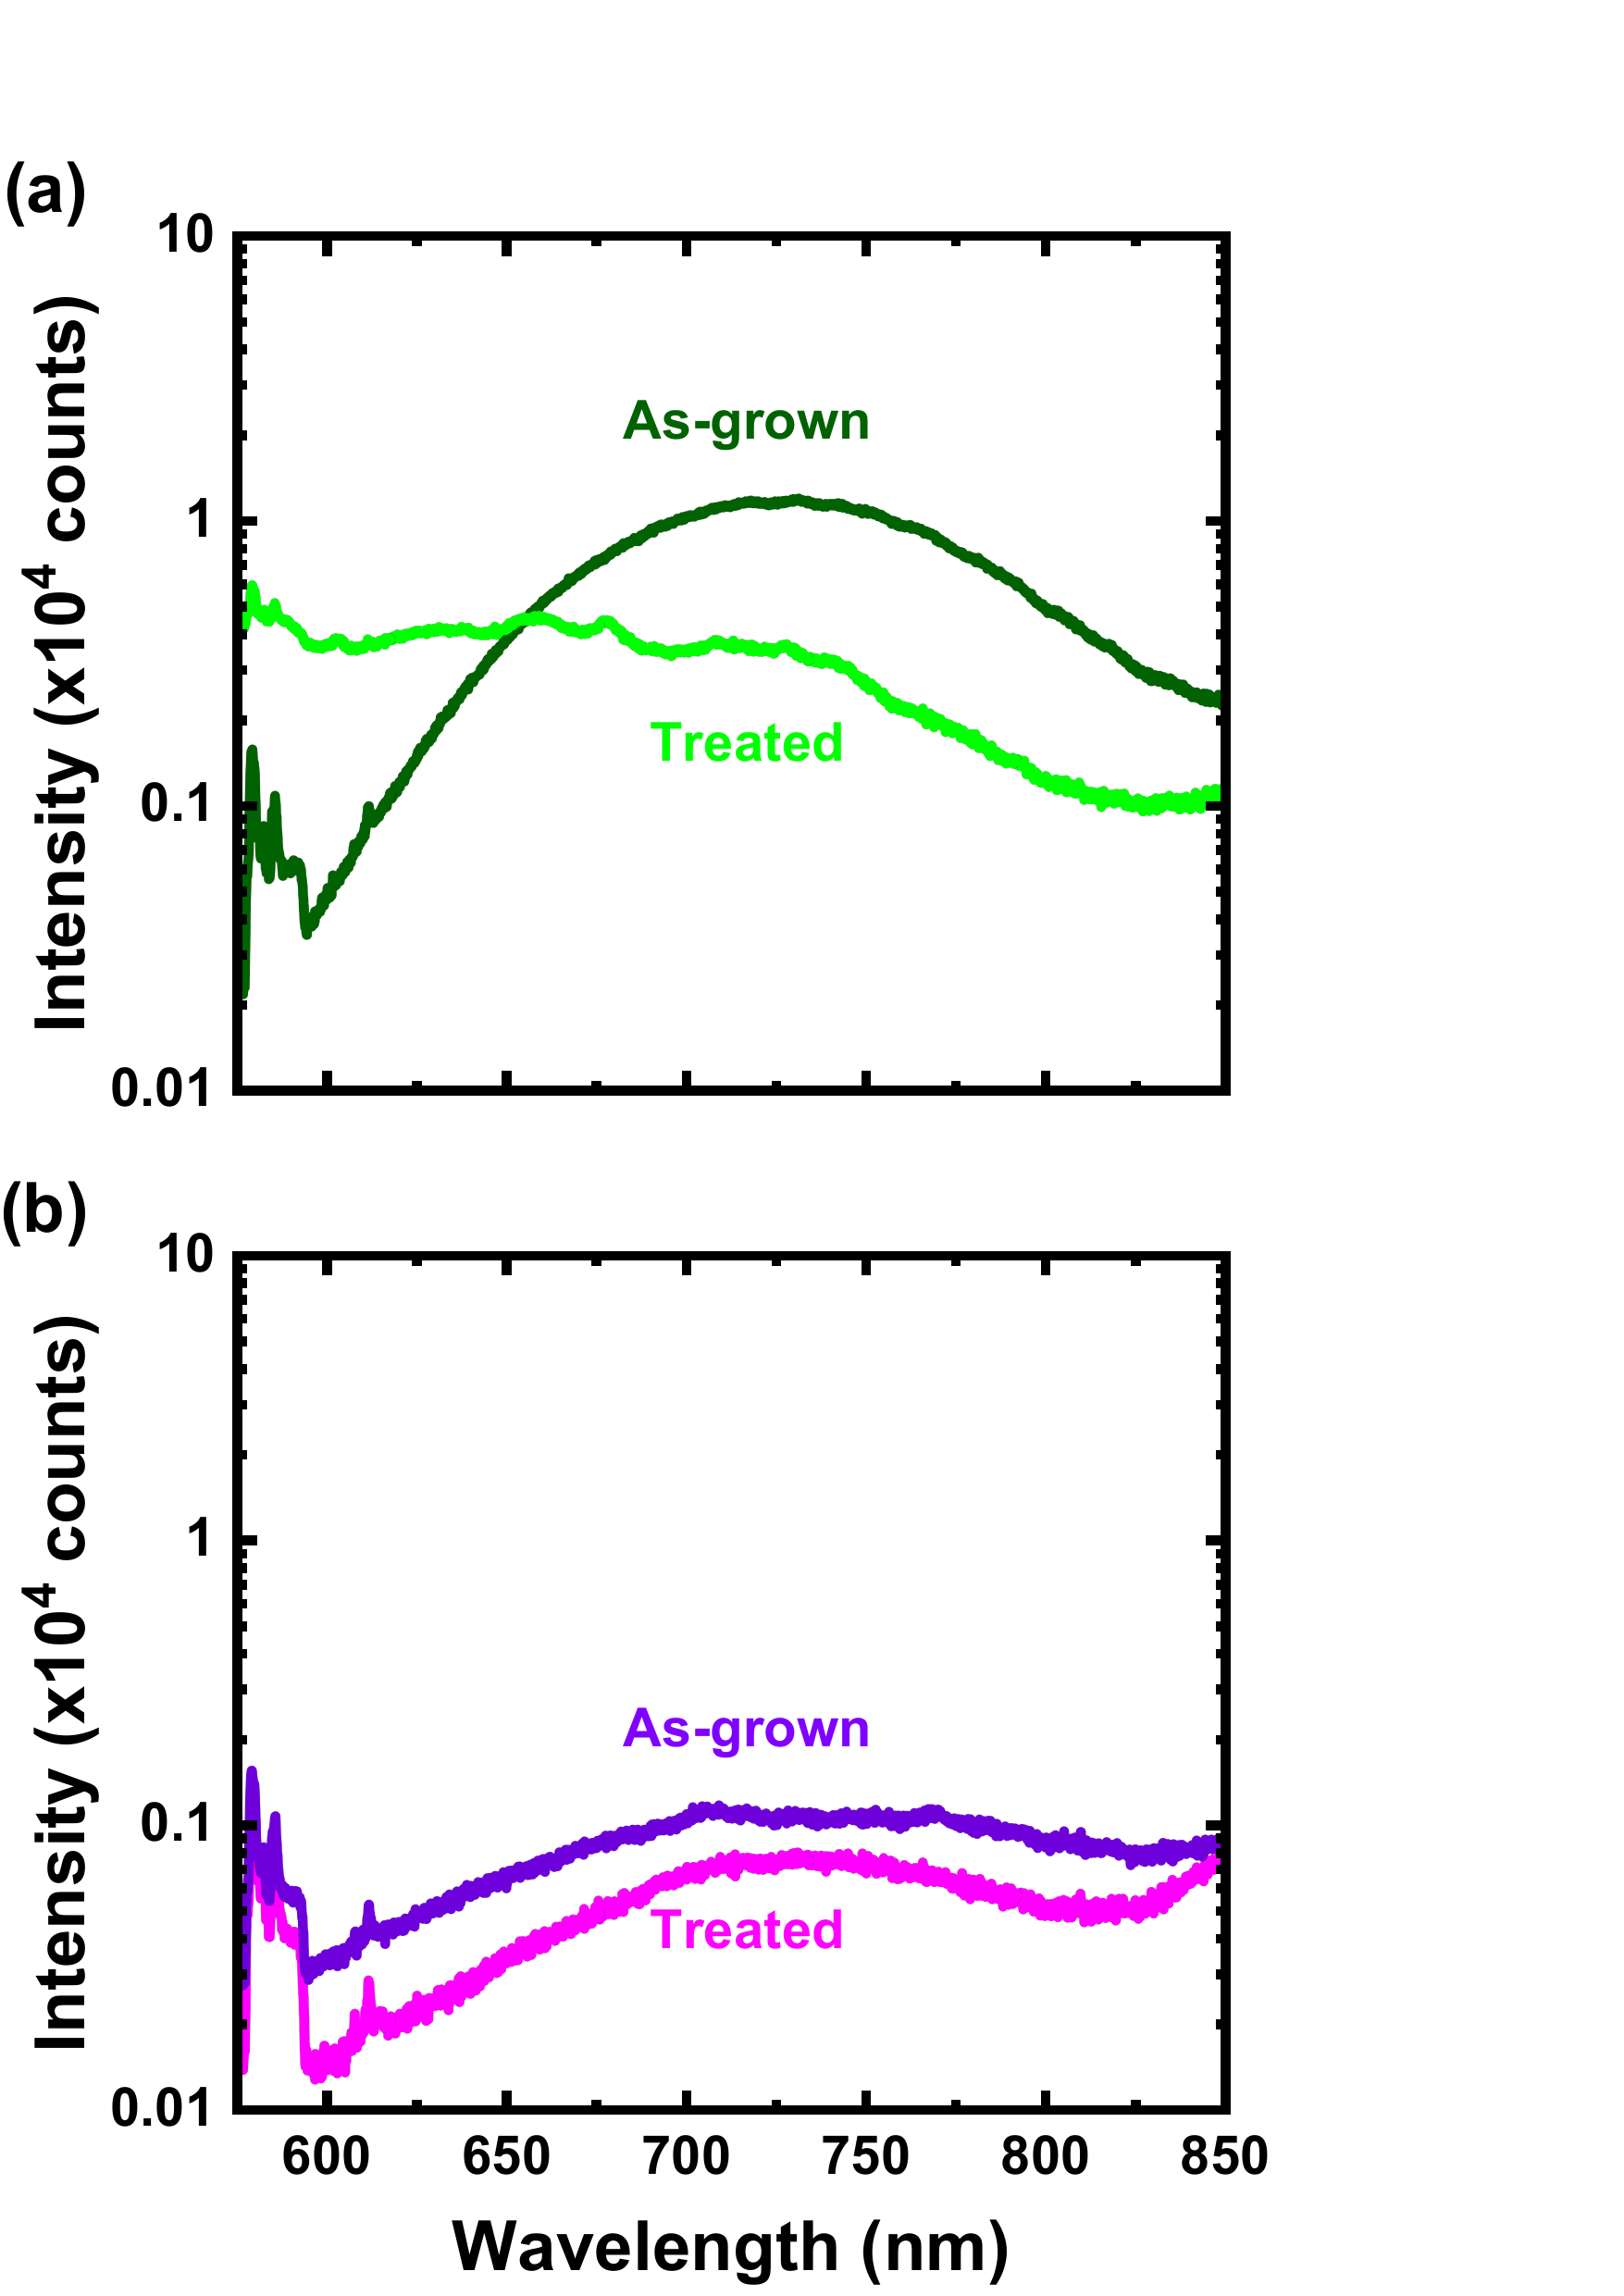}
    \caption{\label{fig:PL_Broad}
    (a) PL spectra of the AlN thin film grown under N-rich conditions, acquired before and after proton irradiation and annealing (dark and bright green curves, respectively).
    (b) Same as panel (a), but for the AlN thin film grown under Al-rich conditions.
    All measurements were performed at room temperature and under the same laser excitation conditions.
    }
\end{figure}



\end{document}
